# Supplementary material for: Measuring Information from Moments
Source: arXiv:2109.00649 source file (2021-09-01)
Supplement: Supplementary file 7 [file Integrability.tex]

\section{Proof of Lemma~\ref{arv}} \label{aae}

Assume that $\BE\left[|X|^{\deg(p)}\right]=\infty$ (so $\deg(p)\ge 1$), and we will show that $\BE\left[|p(X)|\right] = \infty$ too. Let $k\in [\deg(p)-1]$ be the largest integer for which $\BE\left[ |X|^k \right] < \infty,$ and write $p(u)=u^{k+1}q(u)+r(u)$ for a nonzero polynomial $q$ and a remainder $r\in \SP_k.$ By monotonicity of norms, $\BE\left[ |X|^j \right]<\infty$ for every $j\in [k].$ Hence, $r(X)$ is integrable. Therefore, it suffices to prove that $X^{k+1}q(X)$ is non-integrable, which we show next.

Consider the set $\calD = \left\{ u\in \BR ~ ; ~ \left| q(u) \right| < |a| \right\}$ where $a\neq 0$ is the leading coefficient of $q.$ If $q$ is constant, then $\calD$ is empty, whereas if $\deg q \ge 1$ then $|q(u)|\to \infty$ as $|u|\to \infty$ implies that $\calD$ is bounded; in either case, there is an $M\in \BR$ such that $\calD\subset [-M,M].$ Now, writing $1=1_{\calD}+1_{\calD^c},$ we obtain
\begin{equation} \label{aru}
    \BE\left[ |X|^{k+1} |q(X)| \right] \ge |a| ~ \BE\left[ |X|^{k+1} 1_{\calD^c}(X) \right].
\end{equation}
But we also have that
\begin{equation}
    \infty = \BE\left[ |X|^{k+1}\right] \le M^{k+1} +  \BE\left[ |X|^{k+1} 1_{\calD^c}(X) \right],
\end{equation}
so $\BE\left[ |X|^{k+1} 1_{\calD^c}(X) \right]=\infty.$ Therefore, inequality \eqref{aru} yields that $\BE\left[ \left|X^{k+1}q(X)\right|\right]=\infty,$ concluding the proof.
