# Supplementary material for: Measuring Information from Moments
Source: arXiv:2109.00649 source file (2021-09-01)
Supplement: Supplementary file 13 [file a_n.tex]

\subsection{Proof of Inequality \texorpdfstring{\eqref{sx}}{(245)}} \label{aag}

By Lemma~\ref{ii}, 
\begin{equation}
    Q'(y)= \BE[N\mid Y=y] = y - \BE[X \mid Y=y].
\end{equation}
Therefore $X\le M$ implies that, for any constant $z \ge 0,$ we have
\begin{align}
    \int_0^1 \frac{ztQ'(zt)}{\sqrt{1-t^2}} \, dt &= \frac{\pi}{4} z^2 - z \int_0^1 \hspace{-4pt} \frac{t}{\sqrt{1-t^2}}  \frac{\mathbb{E}\left[ X e^{-(X-zt)^2/2} \right]}{ \mathbb{E}\left[e^{-(X-zt)^2/2}\right]} dt \\
    &\ge \frac{\pi}{4} z^2 - Mz.
\end{align}
We have $\pi z^2/4-Mz>n$ for $z=(2M+\sqrt{2})\sqrt{n}.$ Since $y \mapsto yQ'(y)$ is strictly increasing over $(0,\infty)$ (condition~\ref{aam} of Definition~\ref{ig}), we conclude that $a_n(Q)\le (2M+\sqrt{2})\sqrt{n}.$
